# Supplementary material for: Cambricon-LLM: A Chiplet-Based Hybrid Architecture for On-Device Inference of 70B LLM
Source: arXiv:2409.15654 source file (2024-09-24)
Supplement: Supplementary file 1 [file 12_appendix.tex]

% \vspace{-3pt}
\newpage
\onecolumn

\setlength{\parindent}{0pt}

\section{Appendix: summary of change}
\textbf{Revisions in Section I}

Add an NVIDIA client GPU, Jetson Orin, in \autoref*{fig:1_both}(\#B).

\textbf{Revisions in Section II}

Correct expression errors (\#B).

\textbf{Revisions in Section III}

Correct inaccurate descriptions of arithmetic intensity (\#B).

Correct inaccurate expression of page-sized read (\#E).

Add more information about flash error rates (\#C).

\textbf{Revisions in Section IV}

Add more details on SFU (\#D).

Fix the incorrect units "TOPS" (\#C).

\textbf{Revisions in Section V}

Fix a typo in the equations.

\textbf{Revisions in Section VII}

Add area and power overhead of compute core (\#B, \#C, \#E).

\textbf{Revisions in Section VIII}

Add result on the performance of \xname~under W4A16 quantization (\#D).

Add experiment on different tile sizes (\#C).

Add cost analysis (\#C).

% \subsection{Revisions in Section I}
% \noindent Add an NVIDIA client GPU, Jetson Orin, in \autoref*{fig:1_both}(\#B).

% \subsection{Revisions in Section II}
% \noindent Correct expression errors (\#B).

% \subsection{Revisions in Section III}
% \noindent Correct inaccurate descriptions (\#B).
% \noindent Add more information about flash error rates (\#C).

% \subsection{Revisions in Section IV}
% \noindent Fix the incorrect units (\#C).

% \subsection{Revisions in Section V}
% \noindent Fix a typo in the equations.

% \subsection{Revisions in Section VII}
% \noindent Add area and power overhead of compute core (\#B, \#C, \#E).

% \subsection{Revisions in Section VIII}
% \noindent Add result on the performance of \xname~under W4A16 quantization (\#D).

% \noindent Add experiment on different tile sizes (\#C).

% \noindent Add cost analysis (\#C).
